# Supplementary material for: Discrete Auto-regressive Variational Attention Models for Text Modeling
Source: arXiv:2106.08571 source file (2021-06-16)
Supplement: Supplementary file 1 [file appendix.tex]

% \section{Generation Diversity}
% \label{sec:diversity}



% \section{Qualitative Analysis}
% \label{sec:qualitative}
% %\subsubsection{Qualitative Analysis}
% We visualize the generated sentences by Pretraining+FBP VAE, VAE+Attn, GAVAM, and DAVAM in Table~\ref{tab:appendix_sentences}, along with their fluency scores (PPL$\downarrow$) measured by GPT-2~\cite{radford2019language}. 
% As VAE+Attn does not employ an auto-regressive prior, it cannot generate well-correlated latent sequences from uninformative Gaussian distributions, and thus the generated sentences are hardly readable.
% On the other hand, GAVAM is armed with the auto-regressive prior and shows more readable sentences despite poor semantic meanings. 
% This is a result of posterior collapse, as previously shown in Table~\ref{table:density_results}.
% Finally, DAVAM can produce sentences with interpretable meanings and better fluency scores, even when the sequence length is long. This suggests the discrete latent sequence combined with auto-regressive prior enjoys unique advantages in language generation from scratch.


%We list more sentences generated as further qualitative analysis. The accompanied GPT-2 PPL scores for measuring fluency are attached correspondingly. It can be observed pretraining+FBP VAE can produce readable sentences with moderate PPL scores.
%VAE+Attn produces sentences with lots of repeated tokens that are hardly readable, and all of which are associated with poor PPL scores. This is probably due to poorly correlated samples from the uninformative Gaussian prior distribution.
%For GAVAM, despite being slightly better than VAE+Attn, the generated sentences of various lengths are all hardly readable as a result of posterior collapse.
%On the contrary, our DAVAM can produce sentences with understandable meanings and lowest PPL scores, even when the sequence length is long. This suggests latent sequences sampled from the discrete auto-regressive prior indeed contain semantic dependency that benefits language generation.
% accompanied with large PPL



% \begin{table*}[t]
% \begin{center}
% \caption{Sampled short, medium and long sentences as well as their GPT-2 PPL scores for measuring fluency. }
% \footnotesize
% \resizebox{0.98\textwidth}{!}{
% \begin{tabular}{l|l|c}
% % \toprule
% \hline
% Methods & Samples & PPL$\downarrow$ \\\hline
% pretraining &  \tabitem [s] i can say what can be the least in terms also in any form of power stream [/s] & 5.97 \\
% \cdashline{2-3}
% +FBP& \tabitem [s] i hate wandering, i just wan na know when the skies in the sky and the winds. [/s] & 5.64\\
% \cdashline{2-3}
% VAE &\tabitem [s] how you define yourself ? birth control. you will find yourself a dead because of your periods. [/s] & 5.43\\
% \cdashline{2-3}
% & \tabitem [s] where is it that morning when snow on thanksgiving ? what's the next weekend ? dress it!!!! my & 4.97 \\
% & mother was the teen mom and i love her and she just is going to be my show. [/s] & \\ 
% % \cdashline{2-3}
% % & \tabitem [s] is being UNK to become better ? heck the answer to question is to no problem . perhaps & 6.47 \\
% % & you 'll probably get yourself there [/s] & \\
% \cdashline{2-3}
% &\tabitem [s] what is the real mark of a baseball holmes? i started asking a question on a scale by a great & 4.74\\
% & chiropractor but when it comes to the girl i never want to learn it to me. what should i do need a & \\
% & break from town and wan [/s] &  \\
% \cdashline{2-3}
% &\tabitem [s] are they allowed to join (francisco) in \_UNK. giants in the first place.? check out other answers. & 5.21\\
% & do you miss the economy and not taking risks in the merchant form, what would you tell? go to & \\
% &the yahoo home page and ask what restaurants follow this one. [/s] &  \\
% \hline
% VAE+Attn
% & \tabitem [s] explain some make coming you think and represents middle line girl coming. [/s]  & 8.83 \\
% \cdashline{2-3}
% & \tabitem [s] i want that i 'm just boring and \_UNK as 2006, why are worth to know what? [/s]  & 7.34 \\
% \cdashline{2-3}
% & \tabitem [s] there everyone truly truly helps helps helps helps helps helps helps [/s] & 7.29 \\
% \cdashline{2-3}
% & \tabitem [s] who just live this in you to get usual usual help the idea for out to use guess guess thats UNK  & 7.16 \\
% & this for you to use usual files in the UNK [/s] & \\
% \cdashline{2-3}
% % & \tabitem [s] easiest idea real real 's your before a party does a republican brain before does to hear your &7.04 \\
% % &version of the whole ones the way this does not  [/s] &  \\
% % \cdashline{2-3}
% & \tabitem [s] does? why does not find things in \_UNK and i am 5? i am like to find things else and also & 5.99\\
% &know this way to \_UNK when i am not always find a heart fetish when you do?  [/s] &  \\
% \cdashline{2-3}
% & \tabitem [s]  is masterbating masterbating anyone hi fact fact forgive forgive forgive virgin chlorine does & 5.01\\
% &'re hydrogen download 're whats 're does solve 're whats solve 2y germany germany monde&\\ 
% &pourquoi 'm does fun pourquoi 'm 're 'm 're solve 'm does solve pourquoi 'm 'm 'm 'm solve 'm 'm [/s] & \\
% \hline
% GAVAM 
% & \tabitem [s] generally do problems problems, do you have problems [/s]  & 6.57 \\
% \cdashline{2-3}
% & \tabitem [s] when is any one to be punished and your physical with your local with the only one [/s] & 6.13 \\
% \cdashline{2-3}
% & \tabitem [s] plz can you get a UNK envelope in e ? for me for my switched for eachother i would switched to i & 6.50 \\
% & i think  thats . i need to assume . [/s] & \\
% \cdashline{2-3}
% & \tabitem [s] can i believe the inequality different , use taxes for ... . for regards for the points of the number , & 6.20 \\
% & it 's the number [/s] & \\
% \cdashline{2-3}
% & \tabitem [s] what of there actually a 4 to a person or \_UNK to women) its matter!! its its matter!! its matter!& 5.81\\
% &but make something you have a good help. [/s] & \\
% \cdashline{2-3}
% % & \tabitem [s] what is the worst and worst moment and the worst and worst, and a stranger and hugs, and nobody, & 4.68 \\
% % &and i deserve it, and nobody feels awful and i wont worry and worry.  [/s] & \\
% \cdashline{2-3}
% & \tabitem [s] what to do, yoga is there to place and pa? i can definately, but that, you will the best, but the the only &5.18\\
% &amount right? the best range, it though, to do n't do to be to be out, and  [/s] & \\
% \hline
% DAVAM & \tabitem [s] what is the meaning of time management? [/s] & 4.52 \\
% \cdashline{2-3}
% (K=512)& \tabitem [s] how does this affect your blood pressure your hormones are in an unhealthy way? try using it. [/s] & 4.75 \\
% \cdashline{2-3}
% & \tabitem [s] what should you be thankful for thanksgiving dinner and how to get some money with a thanksgiving &4.25\\
% &dinner? [/s] &  \\
% \cdashline{2-3}
% & \tabitem [s]  i 've \_UNK many e-mails. but ca n't find it i am not sure what to expect from the new name? do you & 4.86\\
% & think it is possible to delete my emails from yahoo inbox. [/s] &  \\
% \cdashline{2-3}
% & \tabitem [s] can there have problems to be solved without problems please help i think it 's possible and & 4.52\\
% & do not worry abt it ? yes it has been done ! it is possible. it 's true that it does [/s] & \\
% \cdashline{2-3}
% % & \tabitem [s] what are some of the biggest popular sites that offer political candidates ?  and what is it ? america & 3.93 \\
% % &is one of them and people , that are not politically correct to their own. but this is the official website & \\
% % & of the united states . [/s] & \\
% % \cdashline{2-3}
% & \tabitem [s] is anyone willing to donate plasma if you are allergic to cancer or anything else? probably you can. & 3.87\\
% &i've never done any thing but it is only that dangerous to kill bacteria. i have heard that it doesn't have & \\
% &any effect on your immune system. [/s]  & \\
% \bottomrule
% \hline
% \end{tabular}}
% \end{center}
% \label{tab:appendix_sentences}
% \end{table*}
